# Supplementary material for: A Comprehensive Framework for Predictive Computational Modeling of Growth and Remodeling in Tissue-Engineered Cardiovascular Implants
Source: arXiv:2503.17151 source file (2025-03-21)
Supplement: Supplementary file 1 [file appendix.tex]

\appendix
\section{Appendix}
\label{sec:Appendix}

%%% Local Variables: 
%%% mode: latex
%%% TeX-master: "../main"
%%% End: 
